# Supplementary material for: Complementary Domain Adaptation and Generalization for Unsupervised Continual Domain Shift Learning
Source: arXiv:2303.15833 source file (2023-10-13)
Supplement: Supplementary file 1 [file supplementary.pdf]

# Supplementary Material:
# Complementary Domain Adaptation and Generalization for Unsupervised Continual Domain Shift Learning

Wonguk Cho[1], Jinha Park[2], and Taesup Kim[1]
[1]Graduate School of Data Science, Seoul National University
[2]Department of Electrical and Computer Engineering, Seoul National University
{wongukcho, jhpark410, taesup.kim}@snu.ac.kr

This Supplementary Material provides additional details of the experiments conducted using our CoDAG framework, which are not included in the main paper due to space constraints.

## 1. The Details of the Experimental Settings

We conduct experiments on three datasets: PACS [7], Digits-five [2, 4, 6, 10], and DomainNet [11]. We maintain consistent training steps per epoch across all domains and domain orders for every dataset. We use 50 steps for PACS, 800 steps for Digits-five, and 75 steps for DomainNet. We set the number of training epochs per domain to 60 for both PACS and DomainNet, and to 75 for Digits-five. For distillation loss, we set the balancing parameter $\alpha$ to $0.2$ for PACS and DomainNet, and $0.5$ for Digits-five.

For optimization, we use the SGD optimizer with a weight decay of 0.0005 and a polynomial learning rate scheduler. An initial learning rate is set to 0.01 for both PACS and Digits-five, and 0.005 for DomainNet. The batch size for mini-batch training is set to 64.

For training of PACS and DomainNet, we use the standard augmentation techniques including random cropping, horizontal flipping, color jittering, and grayscaling. For domain adaptation, we use the Mixup [13] method with the mixup hyperparameter set to 2.0.

## 2. The Details of the Network Architecture

Our model network consists of three parts: feature extractor, intermediate module, and classifier. We utilize ResNet-50 [3] as the feature extractor for both PACS and DomainNet, while for Digits-five, we use DTN [8]. ResNet-50 is initialized with the weights pretrained with ImageNet [1].

The intermediate module that connects the feature extractor and classifier is made up of a fully connected layer, a Batch Normalization layer, a ReLU layer, and another fully connected layer. The output dimension of the first fully connected layer is 512 for both PACS and DomainNet, and 256 for Digits-five. The output dimension of the other fully connected layer is 256 for both PACS and DomainNet, and 128 for Digits-five. The classifier consists of a single fully connected layer with weight normalization.

## 3. The Details of the Auxiliary Methods

In this section, we explain the implementation details of the auxiliary methods we employed for the experiments of our CoDAG framework in this paper.

**SHOT** We use simple self-supervised pseudo-labeling, along with information maximization proposed by Liang *et al.* [8]. The balancing parameter $\beta$ is set to $0.1$.

**RandMix** We use the Randmix augmentation implemented by Liu *et al.* [9]. For the samples from target domains, Randmix is applied only for the ones with prediction confidence over $0.5$ for PACS and $0.8$ for Digits-five and DomainNet.

**SelNLPL** To train the DG model using SelNLPL [5] for a given number of training epochs, we divide the epochs equally into three parts for NL, SelNL, and SelPL. For SelPL, $\gamma$ is set to $0.5$.

**Replay buffer** We build the replay buffer based on the iCaRL approach [9, 12]. The prototypes are created for each class in the current domain to prioritize which data to save and remove in the replay buffer based on their proximity to the prototypes.

To accommodate the fixed memory size of the replay buffer, we remove some of the stored samples to make room for new ones, while retaining $M/(K \times t)$ samples for each class in every previous domain, where $M$ is the maximum

Table 1. The list of different domain orders from each dataset for the main experiments, which are referenced from [9].

| Order | PACS | Digits-five | DomainNet |
|---|---|---|---|
| Order 1 | A→C→P→S | SN→MT→MM→SD→US | Re→Pa→In→Cl→Sk→Qu |
| Order 2 | A→C→S→P | SN→SD→MT→US→MM | Cl→In→Pa→Qu→Re→Sk |
| Order 3 | A→P→C→S | MM→US→MT→SD→SN | Cl→Re→In→Qu→Sk→Pa |
| Order 4 | C→A→S→P | MT→MM→SN→SD→US | In→Qu→Cl→Pa→Re→Sk |
| Order 5 | C→S→P→A | MT→MM→US→SN→SD | Pa→Sk→Qu→In→Re→Cl |
| Order 6 | P→A→C→S | SD→MM→SN→MT→US | Qu→Re→Cl→Pa→In→Sk |
| Order 7 | P→S→A→C | SD→SN→US→MM→MT | Qu→Sk→Cl→In→Pa→Re |
| Order 8 | P→S→C→A | SD→US→MM→SN→MT | Sk→In→Pa→Cl→Re→Qu |
| Order 9 | S→C→A→P | US→MT→SN→MM→SD | Sk→Re→Pa→Cl→Qu→In |
| Order 10 | S→P→C→A | US→SD→SN→MM→MT | Sk→Re→Qu→Pa→In→Cl |

number of samples that can be stored in the replay buffer, $K$ is the number of classes, and $t$ represents the number of past domains. In our main experiments, $M$ is set to 200 for all datasets.

# 4. The Details of the Main Experiments

For the main experiments, we use the 10 different orders from each dataset, presented in Table 1, which are randomly selected by [9]. The first domain in a given order is used as a source domain, and the rest are used target domains. For each order, experiments are repeated three times with different seeds (2022, 2023, 2024).

Table 2, 3 and 4 display the experiment results for 10 individual orders from each dataset, respectively. The results of the baseline models are referenced from [9]. These results show that our CoDAG outperforms all other comparison baselines in most of the individual orders across different datasets and metrics.

Notably, in terms of the composite score metric *All*, which assesses the overall performance of the models by averaging TDA, TDG, and FA, our CoDAG outperforms all other baseline models in every order, without exception. These results provide further confirmation of the effectiveness and robustness of our CoDAG framework.

# References


[1] Jia Deng, Wei Dong, Richard Socher, Li-Jia Li, Kai Li, and Li Fei-Fei. Imagenet: A large-scale hierarchical image database. In *2009 IEEE conference on computer vision and pattern recognition*, pages 248–255. Ieee, 2009.

[2] Yaroslav Ganin and Victor Lempitsky. Unsupervised domain adaptation by backpropagation. In *International conference on machine learning*, pages 1180–1189. PMLR, 2015.

[3] K. He, X. Zhang, S. Ren, and J. Sun. Deep residual learning for image recognition. In *2016 IEEE Conference on Computer Vision and Pattern Recognition (CVPR)*, pages 770–778, Los Alamitos, CA, USA, jun 2016. IEEE Computer Society.

[4] Jonathan J. Hull. A database for handwritten text recognition research. *IEEE Transactions on pattern analysis and machine intelligence*, 16(5):550–554, 1994.

[5] Youngdong Kim, Junho Yim, Juseung Yun, and Junmo Kim. Nlnl: Negative learning for noisy labels. In *Proceedings of the IEEE/CVF international conference on computer vision*, pages 101–110, 2019.

[6] Yann LeCun, Léon Bottou, Yoshua Bengio, and Patrick Haffner. Gradient-based learning applied to document recognition. *Proceedings of the IEEE*, 86(11):2278–2324, 1998.

[7] Da Li, Yongxin Yang, Yi-Zhe Song, and Timothy M Hospedales. Deeper, broader and artier domain generalization. In *Proceedings of the IEEE international conference on computer vision*, pages 5542–5550, 2017.

[8] Jian Liang, Dapeng Hu, and Jiashi Feng. Do we really need to access the source data? source hypothesis transfer for unsupervised domain adaptation. In *International Conference on Machine Learning*, pages 6028–6039. PMLR, 2020.

[9] Chenxi Liu, Lixu Wang, Lingjuan Lyu, Chen Sun, Xiao Wang, and Qi Zhu. Deja vu: Continual model generalization for unseen domains. In *The Eleventh International Conference on Learning Representations*, 2023.

[10] Yuval Netzer, Tao Wang, Adam Coates, Alessandro Bissacco, Bo Wu, and Andrew Y Ng. Reading digits in natural images with unsupervised feature learning. 2011.

[11] Xingchao Peng, Qinxun Bai, Xide Xia, Zijun Huang, Kate Saenko, and Bo Wang. Moment matching for multi-source domain adaptation. In *Proceedings of the IEEE/CVF international conference on computer vision*, pages 1406–1415, 2019.

[12] Sylvestre-Alvise Rebuffi, Alexander Kolesnikov, Georg Sperl, and Christoph H Lampert. icarl: Incremental classifier and representation learning. In *Proceedings of the IEEE conference on Computer Vision and Pattern Recognition*, pages 2001–2010, 2017.

[13] Hongyi Zhang, Moustapha Cisse, Yann N. Dauphin, and David Lopez-Paz. mixup: Beyond empirical risk minimization. In *International Conference on Learning Representations*, 2018.

Table 2. Comparison of the performance on the PACS dataset for different state-of-art methods in TDA, TDG, FA, and All. The results are presented for each domain order. The results of the baseline models are referenced from [9]. The best results are highlighted in bold.

| Metric & Orders | | SHOT | SHOT++ | Tent | AdaCon | EATA | L2D | PDEN | RaTP | **Ours** |
|---|---|---|---|---|---|---|---|---|---|---|
| TDA | Order 1 | 86.7 | **89.4** | 84.0 | 85.8 | 86.7 | 84.5 | 83.7 | 85.5 | 88.3 |
| | Order 2 | 87.8 | **89.4** | 82.0 | 81.6 | 85.3 | 83.6 | 83.3 | 87.5 | 87.9 |
| | Order 3 | 88.7 | 88.8 | 82.5 | 82.8 | 85.6 | 82.9 | 79.9 | 85.6 | **89.0** |
| | Order 4 | 89.2 | **91.2** | 88.2 | 88.7 | 89.2 | 84.6 | 83.0 | 87.6 | 89.9 |
| | Order 5 | 85.2 | 85.4 | 88.6 | 86.4 | 88.2 | 80.1 | 78.2 | 85.6 | **89.8** |
| | Order 6 | 83.1 | 85.3 | 75.7 | 78.6 | 79.2 | 75.5 | 74.0 | 83.2 | **86.0** |
| | Order 7 | 66.9 | 69.9 | 74.4 | 74.0 | 73.0 | 71.3 | 71.6 | 75.9 | **80.6** |
| | Order 8 | 64.0 | 68.8 | 72.5 | 73.9 | 72.3 | 68.5 | 69.8 | 74.9 | **80.0** |
| | Order 9 | 91.5 | 92.2 | 69.6 | 77.8 | 73.0 | 83.0 | 82.5 | 89.6 | **92.6** |
| | Order 10 | 75.9 | 83.2 | 69.8 | 69.7 | 70.4 | 74.4 | 72.1 | 91.3 | **91.7** |
| | Avg. | 81.9 | 84.4 | 78.7 | 79.9 | 80.3 | 78.8 | 77.8 | 84.7 | **87.6** |
| TDG | Order 1 | 69.4 | 70.4 | 75.5 | 75.2 | 75.1 | 74.0 | 73.7 | 76.8 | **77.8** |
| | Order 2 | 67.0 | 68.7 | 73.1 | 74.6 | 72.5 | 76.0 | 71.6 | 76.7 | **77.2** |
| | Order 3 | 67.8 | 63.3 | 75.6 | 75.9 | 76.1 | 72.8 | 73.5 | **77.7** | 76.2 |
| | Order 4 | 69.5 | 66.1 | 78.5 | 77.1 | 77.4 | 78.1 | 77.2 | 79.5 | **82.5** |
| | Order 5 | 61.1 | 62.2 | **81.6** | 74.6 | 78.3 | 74.6 | 73.5 | 78.5 | 81.2 |
| | Order 6 | 48.5 | 50.0 | 56.2 | 57.2 | 57.4 | 56.5 | 55.8 | **63.4** | 62.1 |
| | Order 7 | 36.6 | 43.2 | 52.5 | 55.4 | 54.3 | 54.9 | 52.0 | 56.1 | **60.1** |
| | Order 8 | 37.2 | 39.0 | 50.6 | 52.1 | 51.8 | 52.8 | 51.5 | 53.8 | **58.8** |
| | Order 9 | 53.1 | 52.7 | 54.3 | 57.3 | 48.2 | 62.0 | 60.9 | 73.3 | **74.6** |
| | Order 10 | 39.1 | 44.6 | 60.2 | 52.3 | 50.0 | 56.7 | 54.6 | 69.7 | **71.4** |
| | Avg. | 54.9 | 56.0 | 65.8 | 65.2 | 64.1 | 65.8 | 64.4 | 70.6 | **72.2** |
| FA | Order 1 | 73.0 | 78.6 | 89.5 | 90.7 | 91.4 | 85.6 | 85.2 | 87.8 | **91.5** |
| | Order 2 | 72.4 | 82.3 | 79.5 | 77.7 | 83.7 | 80.6 | 77.4 | 79.8 | **86.8** |
| | Order 3 | 81.8 | 78.9 | 88.5 | 89.5 | 90.5 | 84.8 | 78.7 | 87.1 | **91.7** |
| | Order 4 | 76.9 | 77.6 | 83.3 | 84.5 | 87.7 | 77.5 | 77.1 | 83.2 | **89.4** |
| | Order 5 | 82.9 | 86.1 | 89.0 | 88.0 | **90.8** | 76.7 | 76.5 | 84.1 | 90.2 |
| | Order 6 | 79.6 | 84.3 | 81.4 | 80.7 | 83.5 | 71.0 | 70.9 | 86.4 | **87.7** |
| | Order 7 | 65.3 | 80.5 | 78.0 | 78.0 | 74.4 | 75.7 | 75.4 | 78.8 | **83.9** |
| | Order 8 | 58.3 | **83.5** | 73.3 | 74.0 | 73.3 | 72.6 | 72.1 | 74.2 | **83.5** |
| | Order 9 | 86.5 | 88.8 | 74.1 | 79.0 | 76.6 | 78.0 | 78.3 | 87.7 | **91.1** |
| | Order 10 | 72.0 | 89.5 | 73.1 | 73.7 | 74.3 | 73.4 | 71.4 | 89.8 | **91.8** |
| | Avg. | 74.9 | 83.0 | 81.0 | 81.6 | 82.6 | 77.6 | 76.3 | 83.9 | **88.8** |
| All | Order 1 | 76.4 | 79.5 | 83.0 | 83.9 | 84.4 | 81.4 | 80.9 | 83.4 | **85.9** |
| | Order 2 | 75.7 | 80.1 | 78.2 | 78.0 | 80.5 | 80.1 | 77.4 | 81.3 | **84.0** |
| | Order 3 | 79.4 | 77.0 | 82.2 | 82.7 | 84.1 | 80.2 | 77.4 | 83.5 | **85.6** |
| | Order 4 | 78.5 | 78.3 | 83.3 | 83.4 | 84.8 | 80.1 | 79.1 | 83.4 | **87.3** |
| | Order 5 | 76.4 | 77.9 | 86.4 | 83.0 | 85.8 | 77.1 | 76.1 | 82.7 | **87.1** |
| | Order 6 | 70.4 | 73.2 | 71.1 | 72.2 | 73.4 | 67.7 | 66.9 | 77.7 | **78.6** |
| | Order 7 | 56.3 | 64.5 | 68.3 | 69.1 | 67.2 | 67.3 | 66.3 | 70.3 | **74.9** |
| | Order 8 | 53.2 | 63.8 | 65.5 | 66.7 | 65.8 | 64.6 | 64.5 | 67.6 | **74.1** |
| | Order 9 | 77.0 | 77.9 | 66.0 | 71.4 | 65.9 | 74.3 | 73.9 | 83.5 | **86.1** |
| | Order 10 | 62.3 | 72.4 | 67.7 | 65.2 | 64.9 | 68.2 | 66.0 | 83.6 | **85.0** |
| | Avg. | 70.6 | 74.5 | 75.2 | 75.6 | 75.7 | 74.1 | 72.9 | 79.7 | **82.9** |

Table 3. Comparison of the performance on the Digits-five dataset for different state-of-art methods in TDA, TDG, FA, and All. The results are presented for each domain order. The results of the baseline models are referenced from [9]. The best results are highlighted in bold.

| Metric & Orders | | SHOT | SHOT++ | Tent | AdaCon | EATA | L2D | PDEN | RaTP | **Ours** |
|---|---|---|---|---|---|---|---|---|---|---|
| TDA | Order 1 | 84.0 | 87.5 | 71.5 | 77.4 | 76.8 | 85.9 | 81.9 | 89.7 | **95.5** |
| | Order 2 | 91.6 | 94.8 | 77.5 | 76.0 | 76.9 | 91.3 | 89.5 | 90.7 | **95.7** |
| | Order 3 | 81.2 | 79.9 | 70.7 | 75.8 | 76.4 | 85.9 | 86.2 | 87.8 | **91.8** |
| | Order 4 | 73.8 | 79.6 | 59.9 | 64.9 | 65.0 | 77.6 | 75.3 | 86.8 | **90.9** |
| | Order 5 | 79.7 | 84.9 | 59.5 | 65.3 | 65.8 | 79.3 | 78.3 | 87.5 | **91.5** |
| | Order 6 | 87.0 | 92.1 | 80.2 | 80.5 | 81.1 | 89.7 | 89.0 | 90.0 | **93.6** |
| | Order 7 | 89.9 | 91.2 | 80.9 | 82.1 | 83.2 | 87.6 | 85.2 | 91.6 | **92.6** |
| | Order 8 | 89.0 | 91.5 | 80.5 | 80.2 | 82.2 | 88.6 | 85.9 | 89.7 | **92.6** |
| | Order 9 | 48.4 | 48.8 | 48.7 | 55.7 | 55.4 | 74.2 | 70.9 | 85.9 | **91.2** |
| | Order 10 | 61.2 | 62.9 | 57.3 | 58.3 | 57.1 | 82.9 | 80.3 | 87.1 | **91.1** |
| | Avg. | 78.6 | 81.3 | 68.7 | 71.6 | 72.0 | 84.3 | 82.3 | 88.7 | **92.7** |
| TDG | Order 1 | 66.2 | 68.3 | 71.1 | 72.6 | 71.3 | 72.3 | 69.4 | 77.0 | **79.2** |
| | Order 2 | 78.0 | 78.2 | 72.9 | 75.8 | 71.5 | 78.1 | 78.4 | 79.5 | **81.8** |
| | Order 3 | 68.3 | 65.8 | 70.7 | 67.0 | 69.6 | 71.7 | 70.5 | 77.0 | **77.1** |
| | Order 4 | 49.1 | 52.0 | 52.2 | 53.2 | 53.7 | 62.3 | 60.4 | **72.0** | 71.9 |
| | Order 5 | 54.0 | 54.1 | 53.1 | 51.1 | 53.6 | 62.7 | 61.4 | **72.9** | 72.5 |
| | Order 6 | 72.3 | 75.2 | 76.9 | 75.8 | 77.8 | 78.2 | 76.8 | 81.0 | **82.6** |
| | Order 7 | 74.8 | 76.0 | 76.9 | 73.0 | 76.1 | 78.1 | 76.8 | **81.9** | 81.5 |
| | Order 8 | 73.9 | 72.6 | 79.3 | 76.9 | 77.9 | 78.0 | 77.3 | 81.3 | **82.2** |
| | Order 9 | 35.1 | 39.0 | 41.3 | 41.3 | 44.1 | 61.7 | 61.7 | **73.2** | **73.2** |
| | Order 10 | 38.6 | 41.7 | 45.9 | 46.3 | 44.2 | 65.5 | 63.8 | 71.7 | **72.3** |
| | Avg. | 61.0 | 62.3 | 64.0 | 63.3 | 64.0 | 70.9 | 69.7 | 76.8 | **77.4** |
| FA | Order 1 | 60.0 | 67.1 | 67.8 | 75.2 | 76.2 | 75.2 | 71.4 | 83.8 | **87.5** |
| | Order 2 | 73.9 | 75.5 | 82.2 | 82.7 | 83.6 | 81.1 | 79.6 | 87.4 | **89.8** |
| | Order 3 | 70.7 | 71.2 | 72.9 | 80.4 | 85.5 | 85.1 | 81.9 | 90.1 | **91.7** |
| | Order 4 | 56.5 | 65.3 | 50.8 | 59.0 | 58.8 | 72.3 | 70.0 | 82.3 | **85.2** |
| | Order 5 | 77.0 | 79.1 | 61.4 | 71.7 | 71.2 | 74.9 | 73.9 | 85.2 | **87.8** |
| | Order 6 | 59.3 | 67.4 | 81.2 | 80.4 | 79.7 | 76.8 | 74.1 | 84.9 | **86.5** |
| | Order 7 | 62.2 | 71.0 | 79.8 | 82.1 | 80.9 | 77.6 | 76.1 | 84.7 | **86.4** |
| | Order 8 | 57.2 | 66.0 | 80.0 | 81.9 | 79.4 | 75.0 | 72.6 | 83.3 | **85.3** |
| | Order 9 | 25.1 | 30.0 | 33.1 | 56.8 | 61.8 | 72.5 | 68.5 | 85.1 | **86.5** |
| | Order 10 | 39.7 | 52.5 | 51.5 | 52.0 | 52.4 | 74.1 | 72.0 | 82.8 | **84.2** |
| | Avg. | 58.2 | 64.5 | 66.1 | 72.2 | 73.0 | 76.5 | 74.0 | 85.0 | **87.1** |
| All | Order 1 | 70.1 | 74.3 | 70.1 | 75.1 | 74.8 | 77.8 | 74.2 | 83.5 | **87.4** |
| | Order 2 | 81.2 | 82.8 | 77.5 | 78.2 | 77.3 | 83.5 | 82.5 | 85.9 | **89.1** |
| | Order 3 | 73.4 | 72.3 | 71.4 | 74.4 | 77.2 | 80.9 | 79.5 | 85.0 | **86.9** |
| | Order 4 | 59.8 | 65.6 | 54.3 | 59.0 | 59.2 | 70.7 | 68.6 | 80.4 | **82.7** |
| | Order 5 | 70.2 | 72.7 | 58.0 | 62.7 | 63.5 | 72.3 | 71.2 | 81.9 | **83.9** |
| | Order 6 | 72.9 | 78.2 | 79.4 | 78.9 | 79.5 | 81.6 | 80.0 | 85.3 | **87.6** |
| | Order 7 | 75.6 | 79.4 | 79.2 | 79.1 | 80.1 | 81.1 | 79.4 | 86.1 | **86.8** |
| | Order 8 | 73.4 | 76.7 | 79.9 | 79.7 | 79.8 | 80.5 | 78.6 | 84.8 | **86.7** |
| | Order 9 | 36.2 | 39.3 | 41.0 | 51.3 | 53.8 | 69.5 | 67.0 | 81.4 | **83.6** |
| | Order 10 | 46.5 | 52.4 | 51.6 | 52.2 | 51.2 | 74.2 | 72.0 | 80.5 | **82.5** |
| | Avg. | 65.9 | 69.4 | 66.2 | 69.1 | 69.6 | 77.2 | 75.3 | 83.5 | **85.7** |

Table 4. Comparison of the performance on the DomainNet dataset for different state-of-art methods in TDA, TDG, FA, and All. The results are presented for each domain order. The results of the baseline models are referenced from [9]. The best results are highlighted in bold.

| Metric & Orders | | SHOT | SHOT++ | Tent | AdaCon | EATA | L2D | PDEN | RaTP | **Ours** |
|---|---|---|---|---|---|---|---|---|---|---|
| TDA | Order 1 | 68.4 | **70.5** | 59.0 | 60.4 | 60.0 | 59.9 | 60.8 | 68.6 | 70.3 |
| | Order 2 | 69.7 | 66.2 | 28.9 | 66.2 | 65.8 | 56.5 | 54.2 | 72.0 | **74.7** |
| | Order 3 | 72.6 | 73.4 | 65.6 | 68.6 | 69.4 | 54.8 | 52.7 | 66.1 | **74.3** |
| | Order 4 | 51.3 | 53.5 | 54.6 | 52.2 | 52.9 | 57.3 | 55.2 | 61.7 | **67.0** |
| | Order 5 | 68.5 | 70.9 | 60.3 | 60.3 | 58.7 | 56.9 | 55.7 | 64.4 | **74.4** |
| | Order 6 | 63.1 | **65.3** | 51.8 | 52.4 | 55.0 | 49.3 | 50.2 | 56.3 | 63.2 |
| | Order 7 | 47.7 | 48.1 | 50.0 | 50.8 | 51.7 | 41.7 | 40.4 | 58.0 | **59.2** |
| | Order 8 | 72.8 | 73.2 | 67.6 | 71.6 | 70.7 | 64.0 | 63.4 | 67.4 | **76.4** |
| | Order 9 | 74.2 | 75.9 | 67.6 | 71.3 | 69.3 | 61.9 | 62.2 | 72.5 | **76.4** |
| | Order 10 | 71.9 | 72.1 | 31.0 | 67.9 | 71.2 | 59.9 | 61.0 | 66.9 | **74.2** |
| | Avg. | 66.0 | 66.9 | 53.6 | 62.2 | 62.5 | 56.2 | 55.6 | 65.4 | **71.0** |
| TDG | Order 1 | 46.9 | 45.5 | 52.1 | 51.3 | 51.2 | 49.6 | 48.0 | 53.3 | **54.0** |
| | Order 2 | 52.2 | 50.0 | 31.0 | 52.7 | 55.2 | 55.6 | 51.2 | 57.6 | **58.1** |
| | Order 3 | 53.6 | 53.3 | 58.4 | 53.7 | 58.7 | 52.8 | 51.1 | 57.5 | **60.2** |
| | Order 4 | 40.8 | 41.9 | 50.6 | 51.3 | 51.1 | 48.2 | 47.0 | 55.8 | **57.7** |
| | Order 5 | 48.4 | 49.6 | 52.8 | 53.0 | 52.8 | 53.1 | 51.0 | 54.2 | **56.0** |
| | Order 6 | 34.0 | 35.3 | 33.1 | 32.9 | 33.6 | 36.5 | 37.2 | 41.8 | **43.5** |
| | Order 7 | 23.2 | 25.7 | 35.4 | 32.9 | 34.4 | 32.2 | 30.2 | 42.5 | **42.6** |
| | Order 8 | 59.2 | 59.9 | 61.0 | 62.0 | 62.0 | 62.1 | 61.4 | **63.2** | 62.7 |
| | Order 9 | 58.7 | 59.3 | 61.3 | 61.6 | 63.3 | 59.4 | 59.9 | **63.8** | 63.5 |
| | Order 10 | 56.2 | 60.1 | 41.2 | 61.3 | 59.0 | 57.4 | 56.4 | 62.3 | **63.2** |
| | Avg. | 47.3 | 48.1 | 47.7 | 51.3 | 52.1 | 50.7 | 49.3 | 55.2 | **56.2** |
| FA | Order 1 | 61.4 | 66.5 | 67.4 | 67.0 | 64.3 | 63.7 | 61.1 | 67.5 | **70.9** |
| | Order 2 | 64.5 | 68.9 | 34.1 | 62.6 | 65.8 | 48.9 | 46.3 | 70.4 | **74.3** |
| | Order 3 | 62.9 | 67.7 | 65.6 | 66.3 | 69.2 | 45.2 | 43.1 | 64.7 | **72.9** |
| | Order 4 | 42.1 | 65.4 | 56.4 | 53.3 | 52.7 | 41.5 | 39.5 | 57.1 | **66.4** |
| | Order 5 | 60.9 | 68.5 | 58.0 | 56.6 | 57.4 | 51.2 | 48.6 | 62.0 | **72.4** |
| | Order 6 | 61.1 | **66.3** | 52.4 | 49.4 | 54.8 | 48.0 | 46.0 | 53.8 | 63.6 |
| | Order 7 | 42.8 | 51.7 | 48.5 | 48.5 | 47.7 | 37.2 | 36.0 | 55.0 | **57.5** |
| | Order 8 | 61.6 | 67.5 | 71.6 | 72.8 | 73.5 | 58.8 | 55.1 | 63.1 | **74.9** |
| | Order 9 | 67.4 | 77.3 | 76.8 | 76.1 | 76.0 | 66.5 | 65.6 | 76.3 | **82.8** |
| | Order 10 | 60.4 | 69.6 | 30.4 | 65.5 | 66.3 | 61.4 | 60.9 | 64.6 | **72.9** |
| | Avg. | 58.5 | 66.9 | 56.1 | 61.8 | 62.8 | 52.2 | 50.2 | 63.5 | **70.9** |
| All | Order 1 | 58.9 | 60.8 | 59.5 | 59.6 | 58.5 | 57.7 | 56.6 | 63.1 | **65.1** |
| | Order 2 | 62.1 | 61.7 | 31.3 | 60.5 | 62.3 | 53.7 | 50.6 | 66.7 | **69.0** |
| | Order 3 | 63.0 | 64.8 | 63.2 | 62.9 | 65.8 | 50.9 | 49.0 | 62.8 | **69.1** |
| | Order 4 | 44.7 | 53.6 | 53.9 | 52.3 | 52.2 | 49.0 | 47.2 | 58.2 | **63.7** |
| | Order 5 | 59.3 | 63.0 | 57.0 | 56.6 | 56.3 | 53.7 | 51.8 | 60.2 | **67.6** |
| | Order 6 | 52.7 | 55.6 | 45.8 | 44.9 | 47.8 | 44.6 | 44.5 | 50.6 | **56.8** |
| | Order 7 | 37.9 | 41.8 | 44.6 | 44.1 | 44.6 | 37.0 | 35.5 | 51.8 | **53.1** |
| | Order 8 | 64.5 | 66.9 | 66.7 | 68.8 | 68.7 | 61.6 | 60.0 | 64.6 | **71.3** |
| | Order 9 | 66.8 | 70.8 | 68.6 | 69.7 | 69.5 | 62.6 | 62.6 | 70.9 | **74.2** |
| | Order 10 | 62.8 | 67.3 | 34.2 | 64.9 | 65.5 | 59.6 | 59.4 | 64.6 | **70.1** |
| | Avg. | 57.3 | 60.6 | 52.5 | 58.4 | 59.1 | 53.0 | 51.7 | 61.4 | **66.0** |
